# Supplementary material for: On-the-fly Synthesis for LTL over Finite Traces: An Efficient Approach that Counts
Source: arXiv:2408.07324 source file (2024-08-14)
Supplement: Supplementary file 1 [file 10-Appendix.tex]

% \section{Omitted Proofs}\label{appd:proof}

% \section{Environment-first Synthesis}\label{appd:mealy}

\section{Algo Backup (Used for implementation reference and will be deleted in the end.)}
non-recursive version with details about Tarjan's algo
\begin{algorithm}[htbp!]
\caption{On-the-fly \ltlf Synthesis}%\label{alg:main-syn}
\LinesNumbered
\DontPrintSemicolon
\KwIn{\ltlf specification $(\varphi,\X,\Y)_{Moore}$}
\KwOut{Realizable or Unrealizable}

$swin\_state\coloneqq\emptyset$, $ewin\_state\coloneqq\emptyset$\;
$swin\_transition\coloneqq\emptyset$, $ewin\_transition\coloneqq\emptyset$\;
\KwRet $\isRealizable(\varphi,\X,\Y)_{Moore}$\;
\;
\myproc{$\isRealizable(\varphi,\X,\Y)_{Moore}$}
{
  $dfn[S]\coloneqq\{0\}$, $low[S]\coloneqq\{0\}$\;
  $time\coloneqq0$, $cur\coloneqq0$\;
  $dfn[\varphi]\coloneqq low[\varphi]\coloneqq time++$\;
  Init a vector $vec$\;
  $vec.\pushBack(\varphi)$\;

  \While{$cur\geq0$}
  {
    $peek\coloneqq \checkCurrentStatus(vec[cur])$\;
    \If{$peek\neq$\textup{Unknown}}
    {
      $cur\coloneqq cur-1$\;
      \textcolor{red}{to correct: need detect scc here}\;
      \If{$cur<0$}
      {
        \KwRet $(peek=\,$System-winning$)\,?\,$Realizable$\,:\,$Unrealizable\;
      }
      \Else
      {
        $low[vec[cur]]=min\{low[vec[cur]],low[vec[cur+1]]\}$\;
      \Continue\;
      }
    }
    $edge\coloneqq$\;
    \If{$edge=$\textup{Null}}
    {
      \If{$dfn[vec[cur]]=low[vec[cur]]$}
      {
        $scc\coloneqq\emptyset$\;
        \While{$|vec|>cur$}
        {
          $scc.\insert(vec.\back())$\;
          $vec.\popBack()$\;
        }
        $\backwardSearch(scc)$\;
      }
      $cur\coloneqq cur-1$\;
    }
    \Else
    {
      $s\coloneqq\fp{vec[cur],edge}$\;
      \If{$dfn[s]=0$}
      {
        $dfn[s]\coloneqq low[s]\coloneqq time++$\;
        $vec.\pushBack(s)$\;
        $cur\coloneqq cur+1$\;
      }
      \ElseIf{$s\in vec$}
      {
        $low[vec[cur]]\coloneqq min\{low[vec[cur]],low[s]\}$\;
      }
    }
  }
  \KwRet $(\varphi\in swin)\,?\,$Realizable$\,:\,$Unrealizable\;
}
\end{algorithm}
